# Supplementary material for: A Self-Organizing Tensor Architecture for Multi-View Clustering
Source: arXiv:1810.07874 source file (2018-10-18)
Supplement: Supplementary file 1 [file 07-appendix.tex]

\section*{Appendix} \label{sec:Appendix}
\begin{proof}
We can rewrite Eq.~(\ref{eq:P1}) in the vector form as 
\begin{equation}
vec(\mathbf{A} (\mathbf{B} \ast (( \mathbf{B} \ast (\mathbf{A}^{\mathrm{T}} \mathbf{X})) \mathbf{C}))) + vec(\mathbf{D} \mathbf{X}) = vec(\mathbf{E}).
\label{eq:P1_vec}
\end{equation}
% For simplicity, in the following we use the notation $\mathbf{A}_{\mathbf{I}} = \mathbf{I} \otimes \mathbf{A}$, $\mathbf{C}^{\mathrm{T}}_{\mathbf{I}} =  \mathbf{C}^\mathrm{T} \otimes \mathbf{I}$, and $\mathbf{D}_{\mathbf{I}} = \mathbf{I} \otimes \mathbf{D}$.
For simplicity, in the following we use the notation $\mathbf{A}_\mathbf{B} = \mathbf{A} \otimes \mathbf{B}$. Notice that $\mathbf{A}_\mathbf{B} \neq \mathbf{B}_\mathbf{A}$. By using $vec(\mathbf{A} \mathbf{X} \mathbf{B}) = (\mathbf{B}^\mathrm{T}_\mathbf{A}) vec(\mathbf{X}) $ and $\mathbf{x} \ast \mathbf{y} = diag(\mathbf{x})\mathbf{y}$, we have:
\begin{align}
& vec(\mathbf{A} (\mathbf{B} \ast (( \mathbf{B} \ast (\mathbf{A}^{\mathrm{T}} \mathbf{X})) \mathbf{C}))) \nonumber \\
= ~& {\mathbf{I}}_\mathbf{A} vec(\mathbf{B} \ast (( \mathbf{B} \ast (\mathbf{A}^{\mathrm{T}} \mathbf{X})) \mathbf{C})) \nonumber \\
= ~& {\mathbf{I}}_\mathbf{A} ( vec(\mathbf{B}) \ast vec( (\mathbf{B} \ast (\mathbf{A}^{\mathrm{T}} \mathbf{X})) \mathbf{C} ) ) \nonumber \\
= ~& {\mathbf{I}}_\mathbf{A} diag( vec(\mathbf{B}) ) vec( (\mathbf{B} \ast (\mathbf{A}^{\mathrm{T}} \mathbf{X}))\mathbf{C}) \nonumber \\
= ~& {\mathbf{I}}_\mathbf{A} diag( vec(\mathbf{B}) ) \mathbf{C}^{\mathrm{T}}_{\mathbf{I}} vec(\mathbf{B} \ast (\mathbf{A}^{\mathrm{T}} \mathbf{X})) \nonumber \\
= ~& {\mathbf{I}}_\mathbf{A} diag(vec(\mathbf{B})) \mathbf{C}^{\mathrm{T}}_{\mathbf{I}} diag(vec(\mathbf{B})) {\mathbf{I}}_{\mathbf{A}^{\mathrm{T}}} vec(\mathbf{X}).
\label{eq:P1_vec_term1}
\end{align}
\vspace{-1pt}
Similarly, we have $vec(\mathbf{D}\mathbf{X}) = {\mathbf{I}}_\mathbf{D} vec(\mathbf{X})$. Then substitute this and Eq.~(\ref{eq:P1_vec_term1}) into Eq.~(\ref{eq:P1_vec}), we arrive at Theorem \ref{theo:LS}.
\end{proof}
